# Supplementary material for: Phase-field simulations of lithium dendrite growth with open-source software
Source: arXiv:1805.03256 source file (2018-05-08)
Supplement: Supplementary file 1 [file SI_PF.pdf]

# Supporting Information: Phase-field simulations of lithium dendrite growth with open-source software

Zijian Hong and Venkatasubramanian Viswanathan*

*Department of Mechanical Engineering, Carnegie Mellon University, Pittsburgh, Pennsylvania 15213, USA*

E-mail: venkvis@cmu.edu

***Derivation of the modified diffusion equation.*** The diffusion equation is derived starting from the mass conservation law:

$$\frac{\partial C}{\partial t} = -\nabla . J \tag{1}$$

where $C, t$ and $J$ are the volume concentration, evolution time and flux of lithium species, respectively. The lithium species include lithium ion ($\mathrm{Li}^+$) and lithium metal. Note that only lithium species are conserved rather than lithium ion, due to the electrochemical reaction at the interface. The volume concentration $C$ has the contributions from the electrode and electrolyte phases:

$$C = C^l(1 - h(\xi)) + C^s h(\xi). \tag{2}$$

where $C^l$ and $C^s$ are the volume concentration of lithium species in the electrolyte and electrode phases, respectively. $h(\xi)$ is the interpolation function which is given in the main

text. Combining Equations 1 and 2, we can get:

$$\frac{\partial C}{\partial t} = h(\xi)[\frac{\partial C^s}{\partial t} - \frac{\partial C^l}{\partial t}] + \frac{\partial h(\xi)}{\partial t}[C^s - C^l] = -\nabla.J \tag{3}$$

Assuming that the diffusivity of the Li-metal is much smaller than the diffusivity of the lithium ion, the flux of lithium species can be written as:

$$J = -\frac{DC_{Li^+}}{RT}[\nabla\mu + nF\nabla\phi] \tag{4}$$

where $D$ and $C_{Li^+}$ are the diffusivity and volume concentration of $Li^+$, respectively. $R, T, n, F$ are the gas constant, temperature, number of electrons in the ion and Faraday constant, respectively. $\mu$ is the chemical potential of lithium. $\phi$ is the local applied overpotential. Combine Equations 3 and 4 together and divide by the site density of the electrolyte $C^l_m$, one can deduce:

$$h(\xi)[\frac{\partial c^s}{\partial t}\frac{C^s_m}{C^l_m} - \frac{\partial c^l}{\partial t}] + \frac{\partial h(\xi)}{\partial t}[c^s\frac{C^s_m}{C^l_m} - c^l] = \nabla.\frac{Dc_{Li^+}}{RT}[\nabla\mu + nF\nabla\phi] \tag{5}$$

Rewriting equation 5 in terms of chemical potential $\mu$, we get:

$$\chi\frac{\partial \mu}{\partial t} = \nabla.\frac{Dc_{Li^+}}{RT}[\nabla\mu + nF\nabla\phi] - \frac{\partial h(\xi)}{\partial t}[c^s\frac{C^s_m}{C^l_m} - c^l] \tag{6}$$

where the susceptibility factor $\chi = \frac{\partial c^l}{\partial \mu}[1 - h(\xi)] + \frac{\partial c^s}{\partial \mu}h(\xi)\frac{C^s_m}{C^l_m}$.

The molar ratio of electrolyte and electrode phases are related to the chemical potential,[1] given by,

$$c^{l,s} = \frac{exp[\frac{(\mu-\epsilon^{l,s})}{RT}]}{1 + exp[\frac{(\mu-\epsilon^{l,s})}{RT}]} \tag{7}$$

where $\epsilon^{l,s} = \mu^{0l,0s} - \mu^{0N}$ is the difference in the chemical potential of lithium and neutral components on the electrolyte/electrode phase at initial equilibrium state. The lithium ion molar ratio $c_{Li^+}$ is related to the electrolyte molar ratio $c^l$:

$$c_{Li^+} = c^l(1-h(\xi)) = \frac{exp[\frac{(\mu-\epsilon^l)}{RT}]}{1+exp[\frac{(\mu-\epsilon^l)}{RT}]}(1-h(\xi)) \tag{8}$$

Equation 6 can be rearranged to obtain the Equation 3 in the main text:

$$\frac{\partial \mu}{\partial t} = \frac{1}{\chi}[\nabla . \frac{Dc_{Li^+}}{RT}(\nabla\mu + nF\nabla\phi) - \frac{\partial h(\xi)}{\partial t}(c^s \frac{C_m^s}{C_m^l} - c^l)] \tag{9}$$

Note that this equation is identical to model developed by Cogswell[1](see Equation 9 in ref. 1) only when $C_m^s = C_m^l$. This assumption has been explicitly made in the original paper by Plapp[2] in deriving the diffusion equation. However, this is not valid in the present study.

***Parameters used in the simulation*** The electrolyte is assumed to be 1 M $LiPF_6$ dissolved in EC/DMC (1:1 volume ratio) solutions. The kinetic coefficient $L_\eta$ is calculated using the following relationship: $L_\eta = i_0 \frac{V_m \gamma}{F\kappa}$.[1] The barrier height W and gradient coefficient $\kappa$ are related to the surface tension $\gamma$ and the interfacial thickness $\delta$: $W = 12\frac{\gamma}{\delta}$, $\kappa = \frac{3\gamma\delta}{2}$.[1] The site density of the electrolyte can be computed by the density (1.3 g/L) and molar mass (90 g/mol) of the electrolyte. All the parameters used in the current phase-field model are shown in the following table:

Table S1: Phase-field simulation parameters

| Variable name | Symbol | Real value | Normalized value | Source |
|---|---|---|---|---|
| Interfacial mobility | $L_\sigma$ | $2.5 \times 10^{-6} m^3/(J \times s)$ | 6.25 | [ 3] |
| Limiting current | $i_0$ | 3 $mA/cm^2$ | 30 | [ 4] |
| Kinetic coefficient | $L_\eta$ | 0.001/s | 0.001 | Computed |
| Electrons transfered | $n$ | 1 | 1 | - |
| Surface tension | $\gamma$ | 0.556 $J/m^2$ | 0.22 | [ 5] |
| Interface thickness | $\delta$ | 1 $\mu$m | 1 | Estimated |
| Transfer coefficient | $\alpha$ | 0.5 | 0.5 | [ 3] |
| Site density of electrode | $C_m^s$ | $7.64 \times 10^4$ $mol/m^3$ | 76.4 | [ 3] |
| Site density of electrolyte | $C_m^l$ | $1.44 \times 10^4$ $mol/m^3$ | 14.4 | Computed |
| Conductivity of electrode | $\sigma^s$ | $10^7$ S/m | $10^7$ | [ 3] |
| Conductivity of electrolyte | $\sigma^l$ | 1.19 S/m | 1.19 | [ 6] |
| Diffusivity of Lithium ion | D | 3.197 $\times 10^{-10}$ $m^2/s$ | 319.7 | [ 6] |

***Nonlinear dendrite growth kinetics*** The interface movement under an applied overpo-

tential of -0.45 V is tracked by plotting the temporal evolution of order parameter $\xi$ along X-direction, as shown in Figure S1a. A sharp interface is observed where the order parameter changes abruptly from 1 to 0 across the interface, which is due to the fact that the interface thickness is much smaller than the system size. The interface moves by $\sim$30 $\mu$m after 57 s, while a further movement of $\sim$90 $\mu$m is shown after another 51 s. The position of the phase boundary is plotted with respect to time, showing a nearly linear growth before 60 s, followed by a rapid nonlinear growth thereafter (Figure S1b). The interface velocity is further computed, which is almost constant before 60 s and then increases exponentially over time. This clearly demonstrated that the dendrite growth is highly nonlinear, which could deteriorate the performance of the battery almost immediately.

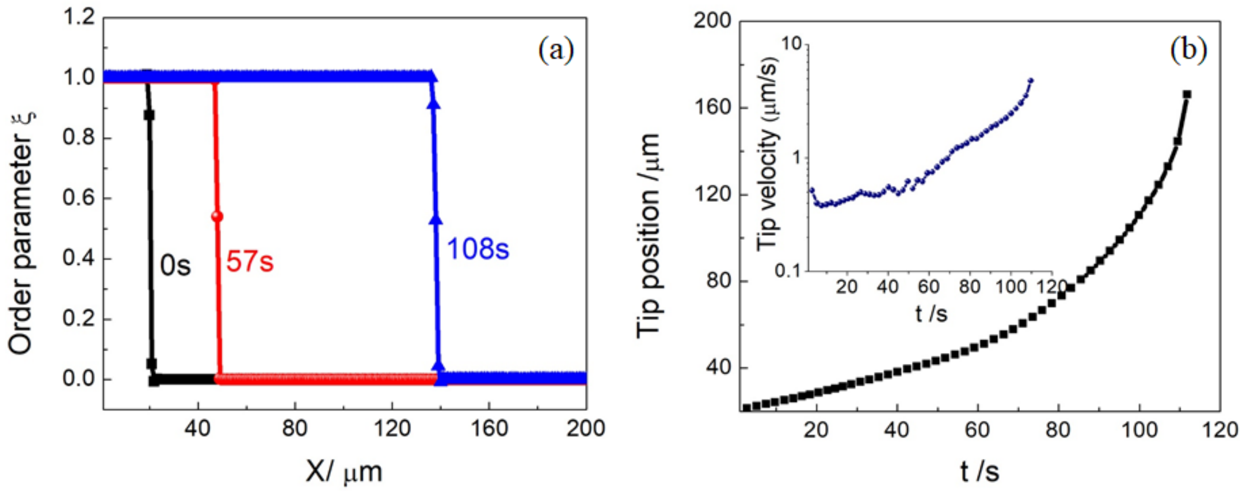


Figure S1: (a) Interface movement (b) and time dependent dendrite growth velocity

The spatial distribution of the electric potential after the formation of dendrites is analyzed in detail (Figure S2). Figure S2a shows the 2-dimensional distribution of the electric potential, which indicates a nearly constant potential at the electrode side (shown in blue), while gradually increases to zero at right boundary deep in the electrolyte. The comparison of the potential distribution between the tip and valley regions is plotted in Figure S2b, which shows a nonlinear potential change near the interfaces of both the valley and tip regions. Meanwhile, the overpotential profile is more flat for the valley region than the tip

region. We further plot the initial electric overpotential distribution along X-direction as a comparison, which gives a linear increase from the electrode/electrolyte interface to the electrolyte (Figure S2d ). Meanwhile, the overpotential distribution along Y-direction (Figure S2c) demonstrates a deep peak for the dendrite tip, resulting in an electric field from the valley to the tip.

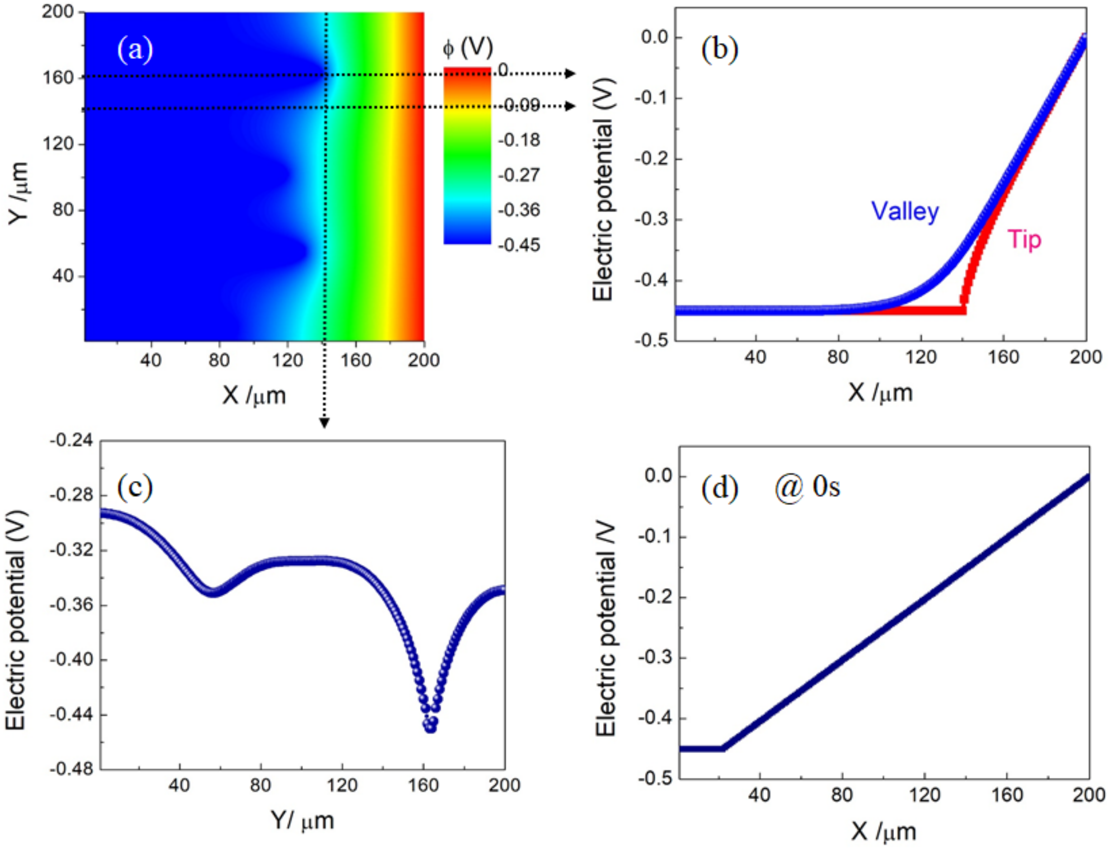


Figure S2: Spatial distribution of electric overpotential (a) potential distribution after the formation of dendrite (b) line plot of the potential distribution for both tip and valley regions (c) line plot of the potential distribution along Y-direction cutting through dendrite tips (d) initial potential distribution along X-direction.

The electric field distribution is calculated by numerical differentiation of the electric potential, as depicted in Figure S3. It can be seen that the electric field in the electrode region is minimal, as the electrode metal has a much larger conductivity than the electrolyte. Interestingly, the electric field near the valley region between the dendrites is also very small, this is consistent with the flat electrical overpotential distribution for the valley region shown

in Figure S2b. The magnified view (Figure S3b) clearly demonstrates that the electric field is highly localized surrounding the dendrite tip, causing strong ion migration from the neighboring regions.

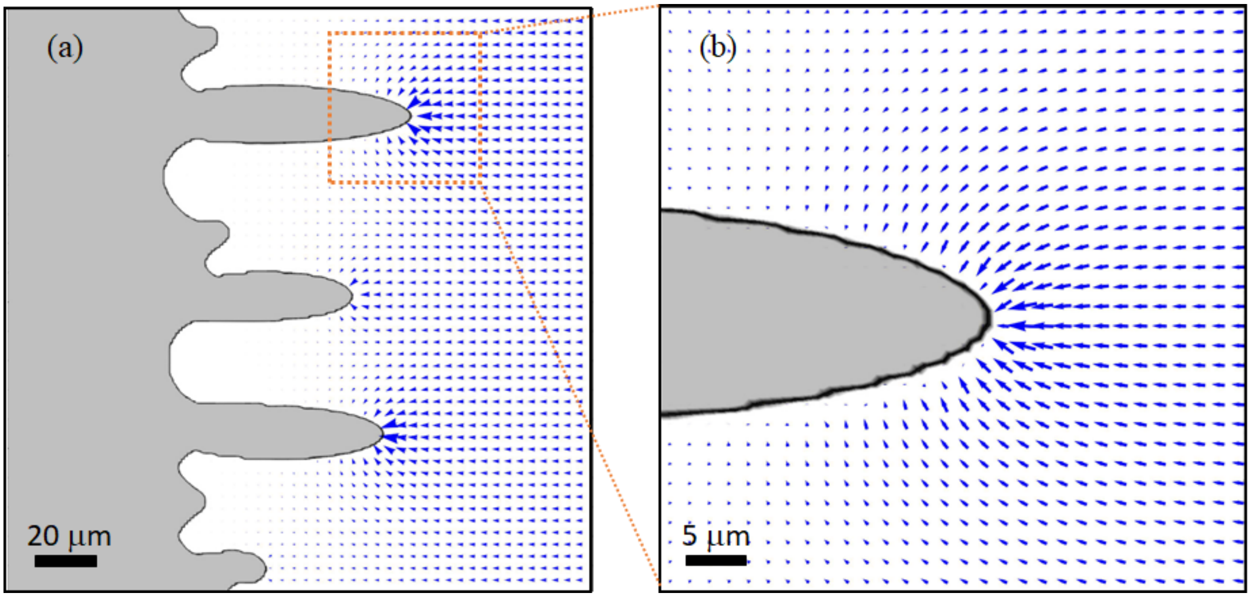


Figure S3: Overlay of electric field vector with the morphology. (a) In the whole simulation volume (b) magnified view in the vicinity of the dendrite tip

***Branching growth kinetics under high overpotential.*** The growth of side branch (tree-like) structures is observed in several previous phase-field studies.[1,3,7] Here, we also show that the side branching can occur at high overpotentials, e.g., -0.5 V (Figure S4). Initially, after 25 s, the interfacial instability shows up, with very fine nuclei. It can be seen that the critical size of the nuclei is much smaller at larger overpotential, which is consistent with experimental observations.[8] This can be easily understood as at higher overpotential, even small perturbation can cause the surface instability and overcome the nucleation barrier. After 45 s, some of the nuclei are growing to form dendrites (Figure S4b), while most of the nuclei growth are hindered. Eventually, only one of these dendrites grow at an overwhelming speed, penetrating through the electrolyte (Figure S4c). Interestingly, with the growth of this long dendrite, some side branches are observed, forming a hyper-branched dendritic structure. The corresponding concentration profile is given in Figures S4(d)-(e). It is shown

that a broad interface is formed similar to the previous case under -0.45 V. After forming the long dendrite, as shown in Figure S4f, a much higher concentration can be found near the dendrite tip.

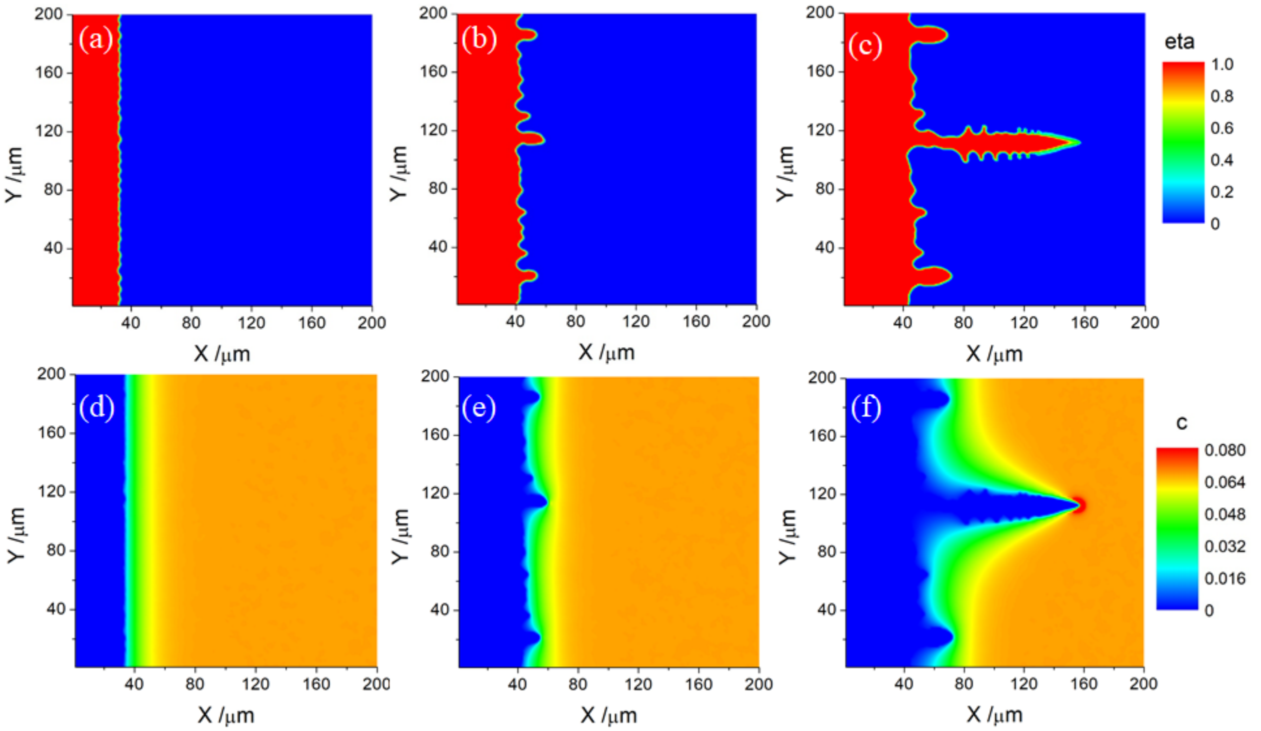


Figure S4: Dynamic morphological evolution under large overpotential of -0.5 V (a) after 25 s (b) after 45 s (c) after 56 s. (d)-(f) the corresponding spatial distribution of Li-ion concentration.

The spatial distributions of applied overpotential and driving force are displayed in Figure S5. The overpotential distribution is almost linear from the electrode/electrolyte interface to electrolyte before the dendrites grow, while a wedge-like distribution is shown after the formation of the long dendrite (Figure S5c). This kind of potential distribution will also give large electric field towards the dendrite tip. The corresponding driving force is plotted in Figures S5 (d)-(f). A larger driving force can be clearly found at the interface regions. While interestingly, after the formation of the long dendrite, the region with side branches also has much larger driving force, indicating that the side branches can also grow larger in this case.

Based on the insights from the simulations, we propose a "compositionally graded solid

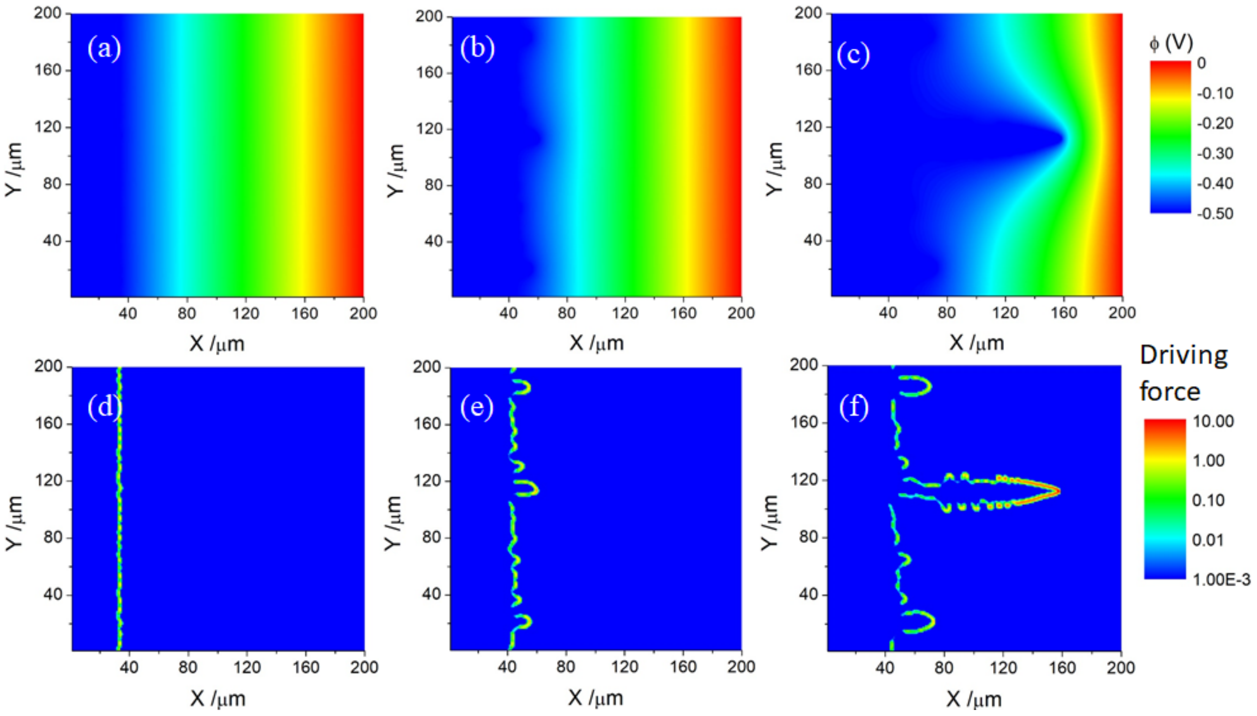


Figure S5: Spatial/temporal distribution of electric potential and driving force at large overpotential. (a)-(c) Evolution of electric potential at 25 s, 45 s and 56 s. (d)-(f) The corresponding spatial distribution of the driving force.

electrolyte" as a potential approach to suppress the dendrite initiation, as shown in Figure S6. The electrolyte can be designed such that it has a higher Li-ion concentration close to the Li-metal anode side while keeping a reasonable relatively lower Li-ion concentration in the vicinity of the cathode side. As the deposition goes on, even if small nuclei are forming, the tip region will have a lower ion concentration than the valley region. Since the reaction rate is directly proportional to the ion concentration, as a result, it can be expected that the electrochemical reaction rate at the tip will be lower than at the valley region, which will prevent the growth of the dendrite at the initial stage. This design may be realized by tuning the doping levels of solid electrolytes (e.g., increasing x in $Li_{7-3x}Al_xLa_3Zr_2O_{12}$ from the anode to cathode), or by varying the lithium containing ceramic to polymer ratio.

***Supplementary videos available.***

Supplementary video 1: Dendrite growth under an applied overpotential of -0.45 V.

Supplementary video 2: Corresponding Lithium-ion concentration evolution @-0.45 V.

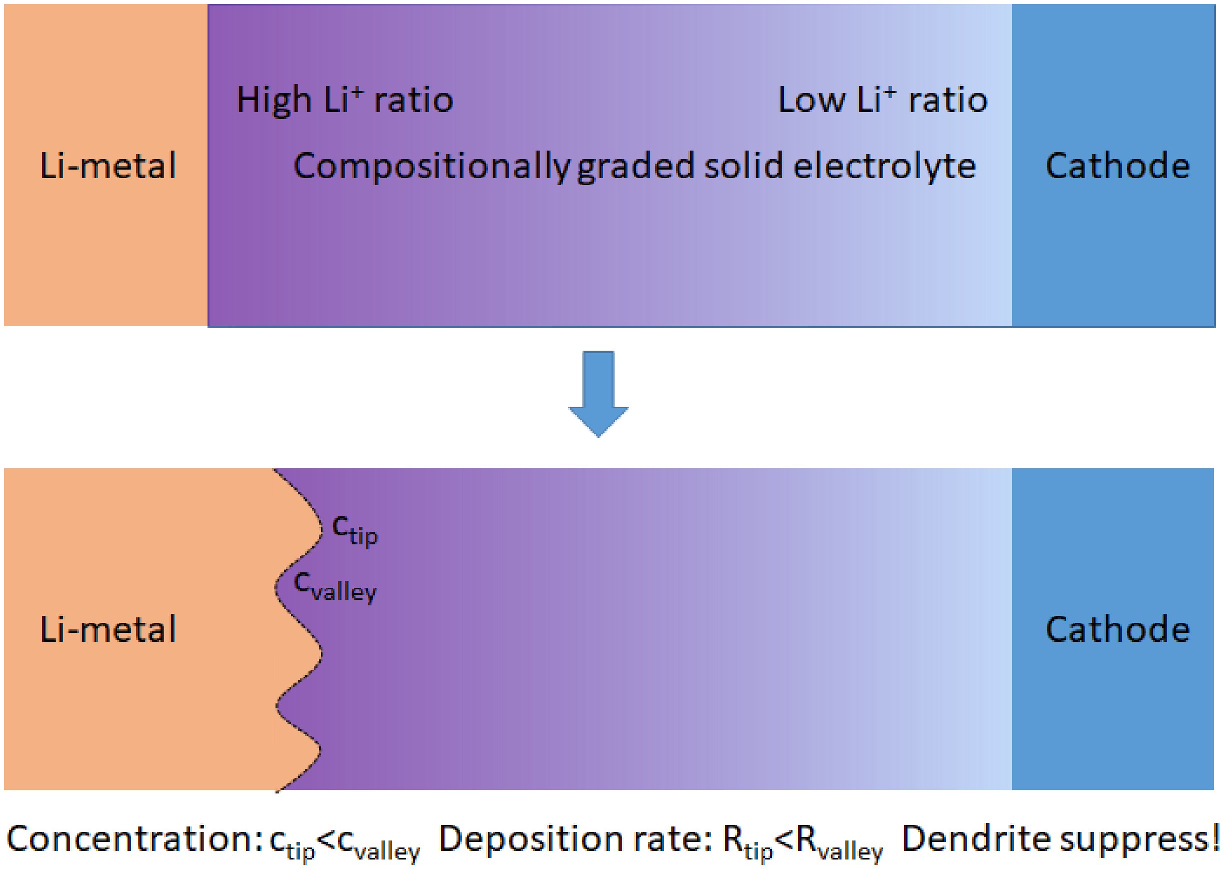


Figure S6: Schematics of the proposed design “compositionally graded solid electrolyte”

Supplementary video 3: Stable deposition under an applied overpotential of -0.32 V.

Supplementary video 4: Corresponding Lithium-ion concentration evolution @-0.32 V.

# References


(1) Cogswell, D. A. Quantitative phase-field modeling of dendritic electrodeposition. *Phys. Rev. E* **2015**, *92*, 011301.

(2) Plapp, M. Unified derivation of phase-field models for alloy solidification from a grand-potential functional. *Phys. Rev. E* **2011**, *84*, 031601.

(3) Chen, L.; Zhang, H. W.; Liang, L. Y.; Liu, Z.; Qi, Y.; Lu, P.; Chen, J.; Chen, L.-Q. Modulation of dendritic patterns during electrodeposition: A nonlinear phase-field model. *J. Power Sources* **2015**, *300*, 376 – 385.

(4) Monroe, C.; Newman, J. Dendrite Growth in Lithium/Polymer Systems: A Propagation Model for Liquid Electrolytes under Galvanostatic Conditions. *J. Electrochem. Soc.* **2003**, *150*, A1377–A1384.

(5) Vitos, L.; Ruban, A.; Skriver, H.; KollÃąr, J. The surface energy of metals. *Surf. Sci.* **1998**, *411*, 186 – 202.

(6) Valøen, L. O.; Reimers, J. N. Transport Properties of LiPF6-Based Li-Ion Battery Electrolytes. *J. Electrochem. Soc.* **2005**, *152*, A882–A891.

(7) Yurkiv, V.; Foroozan, T.; Ramasubramanian, A.; Shahbazian-Yassar, R.; Mashayek, F. Phase-field modeling of solid electrolyte interface (SEI) influence on Li dendritic behavior. *Electrochim. Acta* **2018**, *265*, 609 – 619.

(8) Pei, A.; Zheng, G.; Shi, F.; Li, Y.; Cui, Y. Nanoscale Nucleation and Growth of Electrodeposited Lithium Metal. *Nano Lett.* **2017**, *17*, 1132–1139.
